# Supplementary material for: DeepTensor: Low-Rank Tensor Decomposition with Deep Network Priors
Source: arXiv:2204.03145 source file (2022-04-07)
Supplement: Supplementary file 1 [file appendix.tex]

\section{Hardware}

All the experiments in the main script have been performed on a desktop with 128G of RAM, Intel(R) Core(TM) i7-6850K (3.60GHz, 6 cores, 12 threads and 15MB of cache) CPU and GeForce GTX 1080TI GPU with 12G of memory.

\section{Networks Architectures}

The Deep Decoder architecture \cite{heckel2018deep}. The deep decoder is tasked with converting multiple noise channels into a structured signal using $1x1$ convolutional layers, ReLU and upsampling successively. On the other hand, the Deep Image Prior.

The Deep Image Prior architecture \cite{ulyanov2018deep}. It is a U-Net type “hourglass” architecture with skip-connections with same spatial size for input and output (as opposed to the Deep Decoder that has smaller spatial size inputs than outputs). The default architecture has two million parameters.
